# Supplementary material for: Search for Concepts: Discovering Visual Concepts Using Direct Optimization
Source: arXiv:2210.14808 source file (2022-10-25)
Supplement: Supplementary file 1 [file 08_Appendix.tex]

\section{Appendix}
